# Supplementary material for: Synthetic Semimetals with van der Waals Interfaces
Source: arXiv:2001.09777 ancillary file (2020-01-27)
Supplement: Supplementary file 1 [file Supporting_information_resub.pdf]

# Supporting Information

## Synthetic Semimetals with van der Waals Interfaces

Bojja Aditya Reddy,<sup>†,‡,§</sup> Evgeniy Ponomarev,<sup>†,‡,§</sup> Ignacio Gutiérrez-Lezama,<sup>†,‡</sup>

Nicolas Ubrig,<sup>†,‡</sup> Céline Barreteau,<sup>†,¶</sup> Enrico Giannini,<sup>†</sup> and Alberto F.

Morpurgo<sup>\*,†,‡</sup>

<sup>†</sup>*Department of Quantum Matter Physics, University of Geneva, 24 Quai Ernest  
Ansermet, CH-1211 Geneva, Switzerland*

<sup>‡</sup>*Group of Applied Physics, University of Geneva, 24 Quai Ernest Ansermet, CH-1211  
Geneva, Switzerland*

<sup>¶</sup>*Université Paris Est Creteil, CNRS, ICMPE, UMR 7182, F-94320, Thiais, France*

<sup>§</sup>*These two authors contributed equally*

E-mail: [alberto.morpurgo@unige.ch](mailto:alberto.morpurgo@unige.ch)

### S1. Methods

*Interface Fabrication.* The fabrication of interfaces discussed in the main text is based on the so-called dry-transfer assembly technique. Thin layers – ranging from monolayer (1L) to six-layers (6L) – of SnSe<sub>2</sub> (purchased from 2D semiconductor), ZrS<sub>2</sub> (grown in-house) and WSe<sub>2</sub> (purchased from HQ Graphene) are obtained by mechanical exfoliation of bulk crystals onto Si/SiO<sub>2</sub> substrates. The interfaces are assembled by picking-up these layers and releasing them at a desired location, using polymer-based stamps.<sup>1</sup> The process is done with the aid of a motorized stage under an optical microscope in a nitrogen-filled glove box

(< 0.1 ppm O<sub>2</sub> and H<sub>2</sub>O) in order to avoid any material degradation. In some devices the individual layers forming the interface were intentionally arranged to enable the characterization of both the interface and the layers themselves, as discussed in the main text (Fig. 1(c,d)).

*IL FET Fabrication.* Ionic liquid field effect transistors are realized using conventional microfabrication techniques. The source and drain contacts (Pt/Au), the voltage probes, the reference electrodes and the large planar gate electrodes are fabricated with electron beam lithography, electron-beam evaporation and lift-off. Finally a droplet of ionic liquid (1-butyl-1-methylpyrrolidiniumtris(penta-fluoroethyl) trifluorophosphate [P14][FAP]) is applied on the device covering the whole structure.

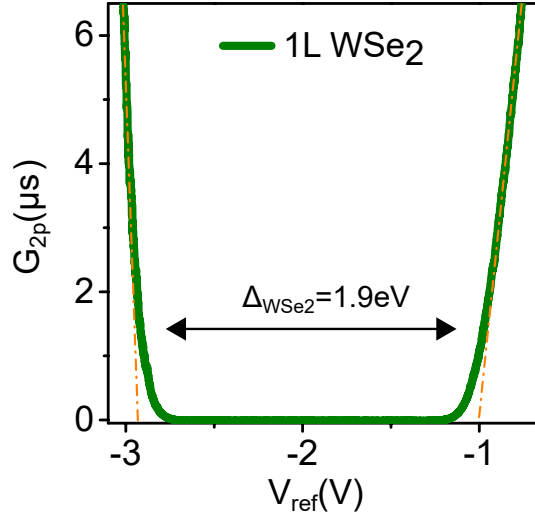

Figure S1: Two terminal conductance ( $G_{2p}$ ) as a function of reference voltage ( $V_{ref}$ ) measured on a 1L-WSe<sub>2</sub> device (the device whose data are shown in Fig. 2(e)). The red dash-dotted lines denote the electron and hole threshold voltages. The difference between these voltages yields the precise value of the band gap of 1L WSe<sub>2</sub>.

## S2. FET transfer curve of 1L WSe<sub>2</sub>

The IL FET transfer curves discussed in the main text are represented as a function of gate

voltage  $V_G$ . For the precise determination of semiconductor band gap, however, it is required to measure conductance as a function of reference voltage, i.e., as a function of the voltage probed with an additional electrode immersed in the ionic liquid. The reason is that the reference electrode accounts only for voltage drop occurring at the FET channel/IL interface and eliminates any possible drop at the gate/IL interface. Fig. S1 shows the two terminal conductance of a WSe<sub>2</sub> monolayer, for the device whose data are plotted in Fig. 2(e), as a function of reference voltage. By doing this, the value of the band gap extracted as the difference between electron and hole threshold voltages is  $\Delta_{WSe_2} = 1.9$  eV, which matches very well previously reported values.<sup>2,3</sup>

### S3. Electronic transport properties of as-exfoliated SnSe<sub>2</sub> layers

As discussed in the main text, the transport properties of our WSe<sub>2</sub>/SnSe<sub>2</sub> interfaces differ from those of their constituents, which are large band gap semiconductors. As the semiconductor character of WSe<sub>2</sub> is widely reported in the literature, and clearly seen in our work by the presence of a gap, it will not be addressed here any further. Instead, we discuss the electronic transport properties of the less studied, as-exfoliated SnSe<sub>2</sub> layers (in the absence of ionic liquid), which we find to be consistent with previous work reported in the literature<sup>4</sup>. Fig. S2 shows the typical transport behaviour of SnSe<sub>2</sub>, illustrated by temperature and magnetic field measurements performed on the 4L-crystal employed in the fabrication of the interface shown in Fig. 4(a) (the layer is protected by a 1L-hBN crystal). As shown in Fig. S2(a), the as-exfoliated layers show a finite conduction at room temperature due to unintentional doping (in line with the electron doping found in Fig. 4(b) at  $V_G = 0$  V). Cooling down SnSe<sub>2</sub>, however, results in an exponential increase of the square resistance at low temperature, which is not observed in our interfaces (see Fig. 5(c)). Furthermore, measurements of the Hall resistance shown in Fig. S2(b) show that conduction in SnSe<sub>2</sub> is due to electrons down to 5K. Conduction is always due to one type of charge carrier, unlike what we find in WSe<sub>2</sub>/SnSe<sub>2</sub> interfaces, where a change of sign in the Hall resistance is observed

as the temperature is decreased (signaling a change from hole to electron conduction). These results clearly show that SnSe<sub>2</sub> by itself cannot be responsible for the semimetallic behaviour observed in WSe<sub>2</sub>/SnSe<sub>2</sub> interfaces.

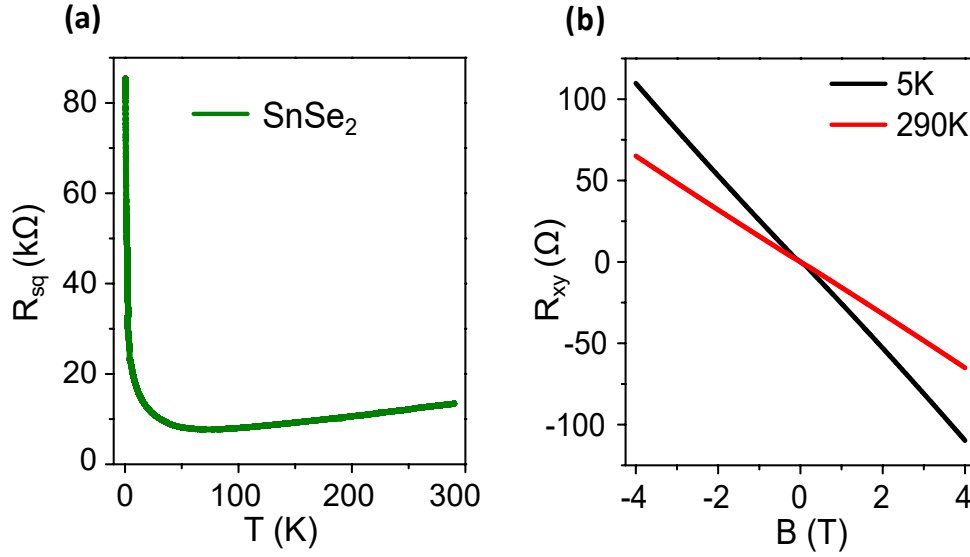

Figure S2: Electronic transport properties of the 4L as-exfoliated SnSe<sub>2</sub> crystal used in the fabrication of the interface shown in Fig. 4(a). (a) Temperature dependence of longitudinal square resistance ( $R_{sq}$ ), showing an exponential increase at low temperature. (b) Transverse resistance ( $R_{xy}$ ) as a function of magnetic field ( $B$ ) measured at two different temperatures, 290K and 5K. The Hall slope is negative signaling that transport in SnSe<sub>2</sub> at all temperatures is due to electrons.

## References

- (1) Zomer, P. J.; Dash, S. P.; Tombros, N.; van Wees, B. J. A transfer technique for high mobility graphene devices on commercially available hexagonal boron nitride. *Applied Physics Letters* **2011**, *99*, 232104.
- (2) Ponomarev, E.; Ubrig, N.; Gutiérrez-Lezama, I.; Berger, H.; Morpurgo, A. F. Semiconducting van der Waals Interfaces as Artificial Semiconductors. *Nano Letters* **2018**, *18*, 5146–5152.
- (3) Zhang, H.; Berthod, C.; Berger, H.; Giamarchi, T.; Morpurgo, A. F. Band Filling and Cross Quantum Capacitance in Ion-Gated Semiconducting Transition Metal Dichalcogenide Monolayers. *Nano Letters* **2019**, *19*, 8836–8845.
- (4) Zeng, J.; Liu, E.; Fu, Y.; Chen, Z.; Pan, C.; Wang, C.; Wang, M.; Wang, Y.; Xu, K.; Cai, S. et al. Gate-Induced Interfacial Superconductivity in 1T-SnSe<sub>2</sub>. *Nano Letters* **2018**, *18*, 1410–1415.
